# Supplementary material for: Entanglement-Optimal Trajectories of Many-Body Quantum Markov Processes
Source: arXiv:2111.12048 source file (2022-05-16)

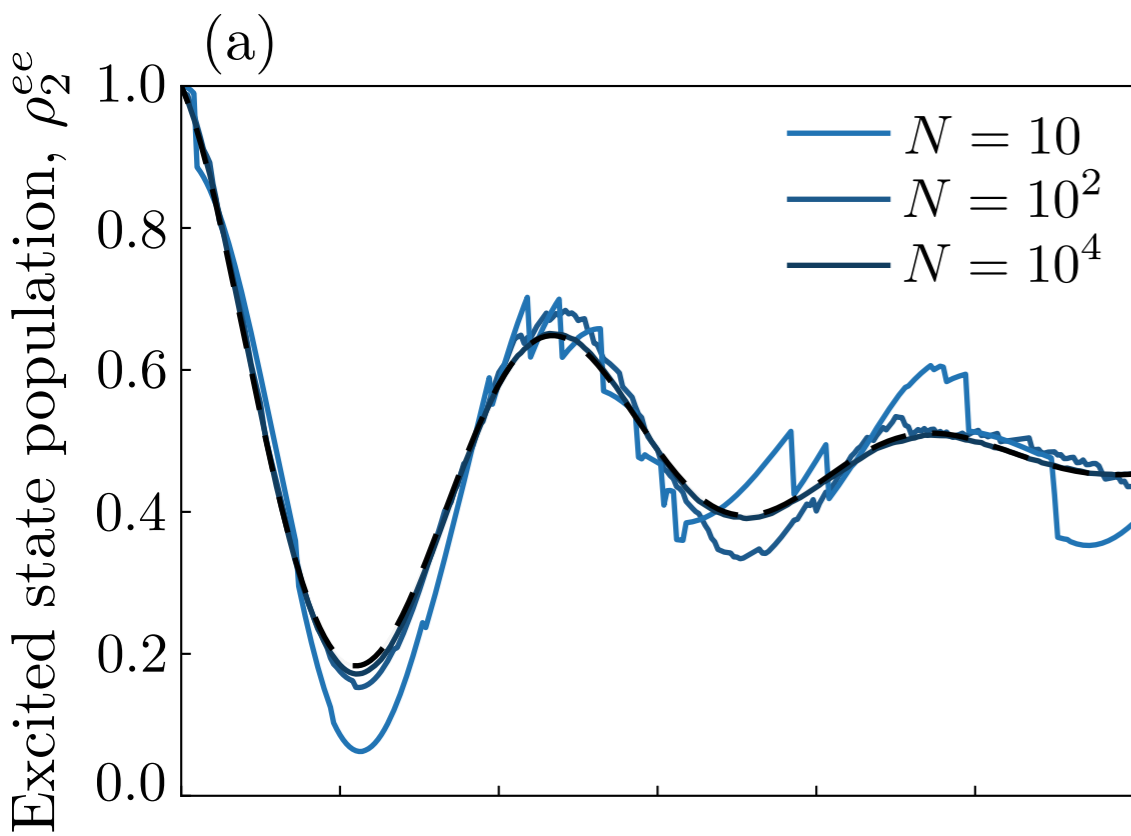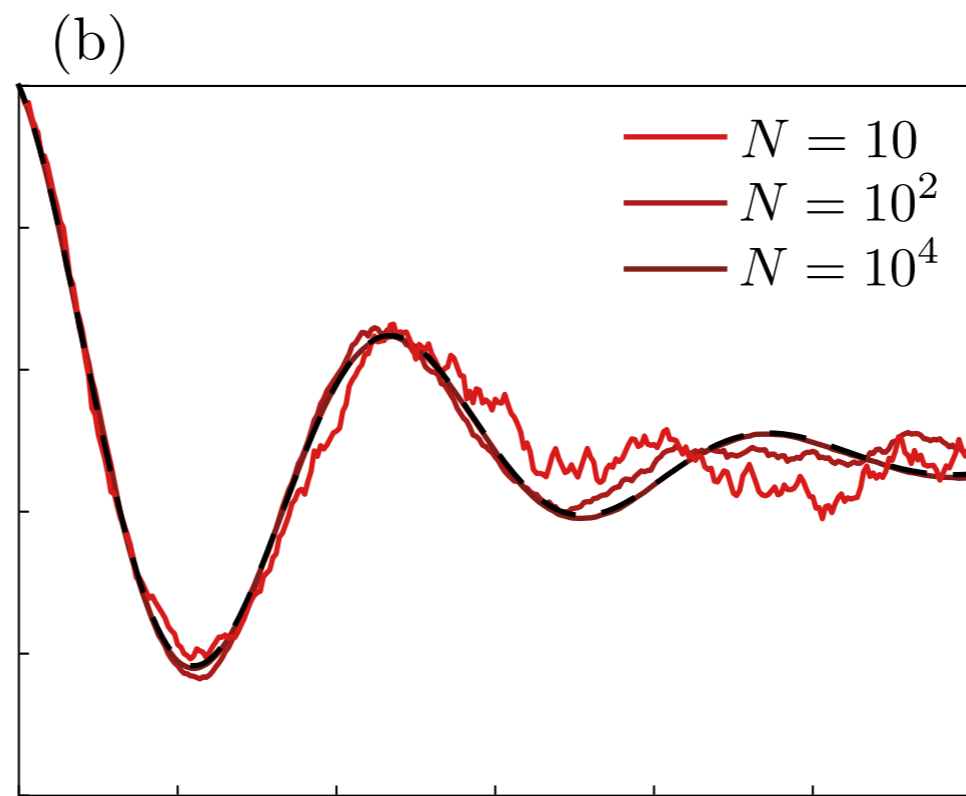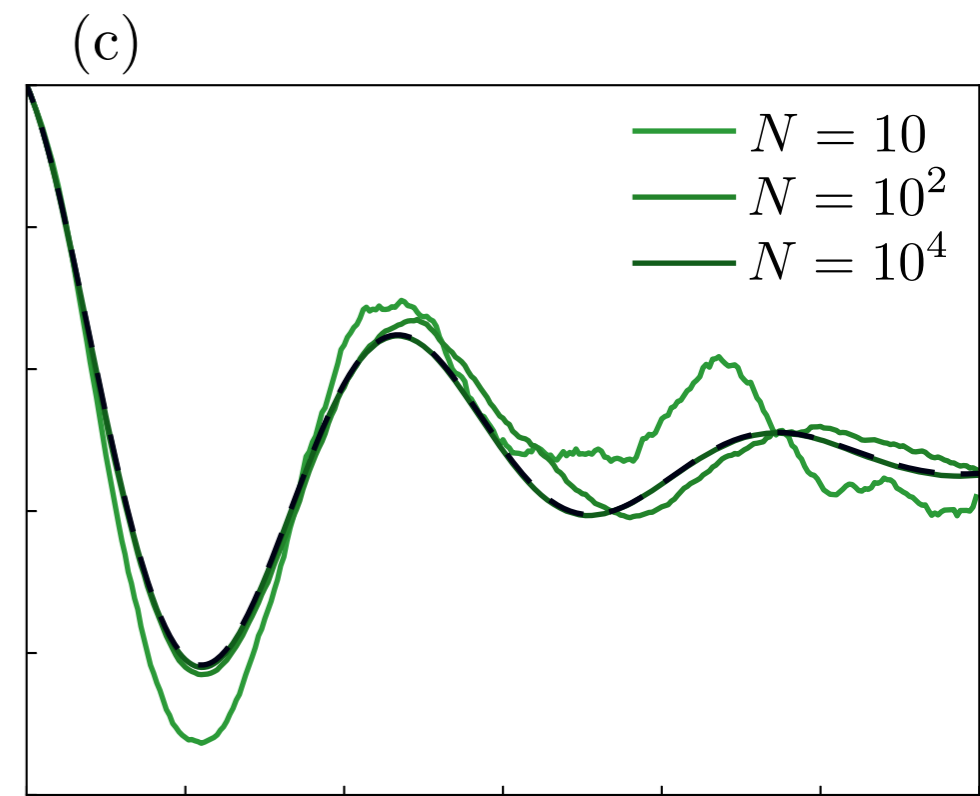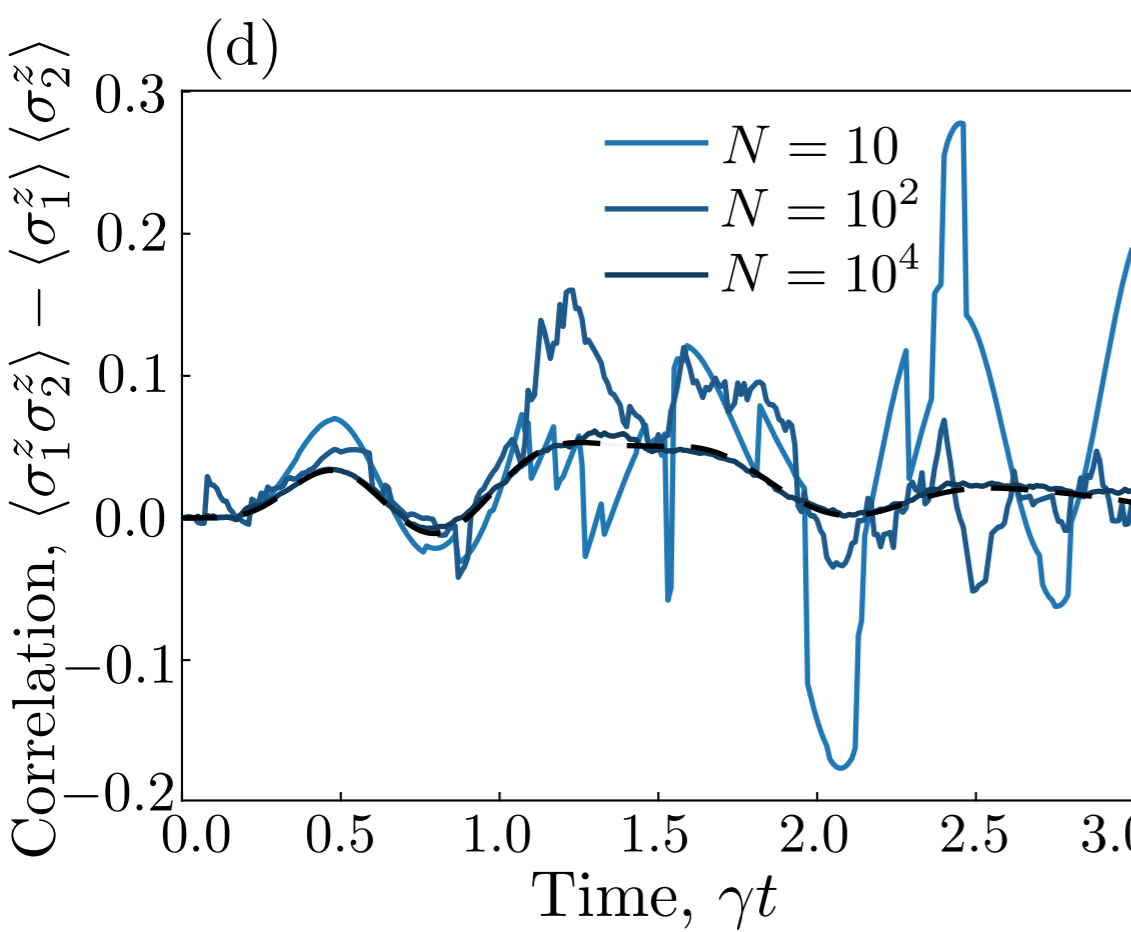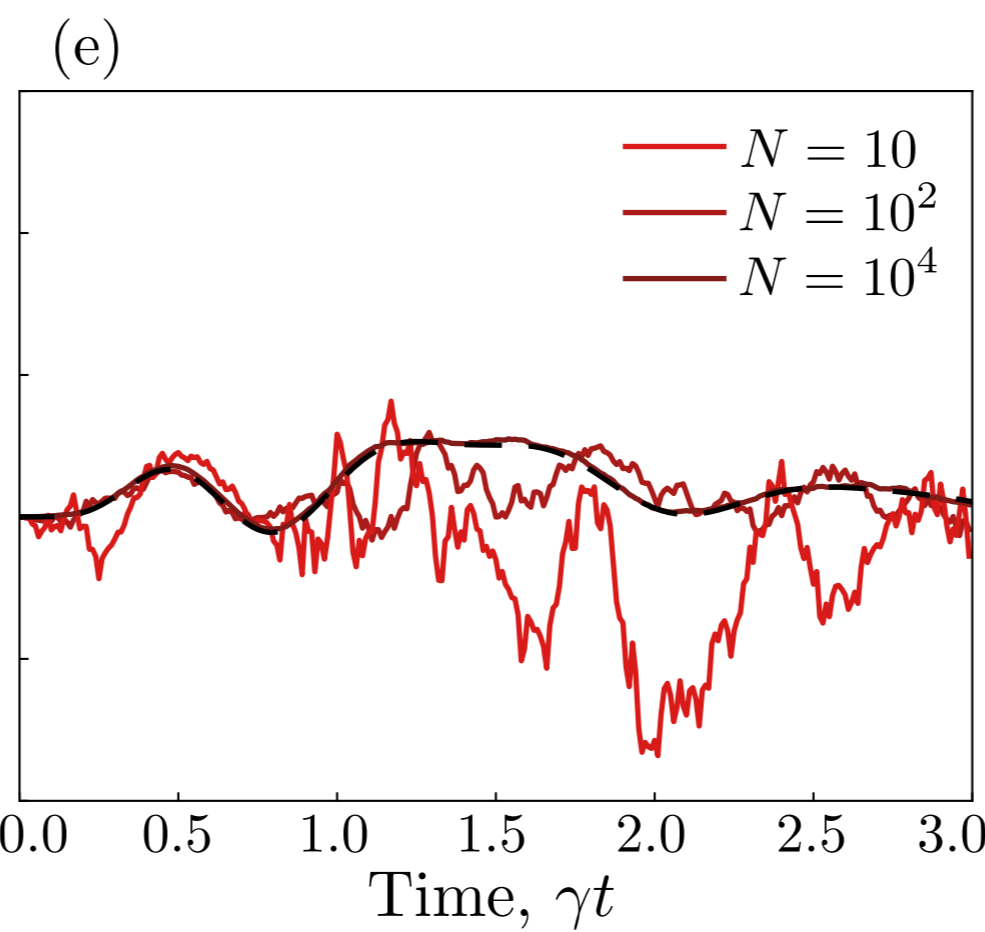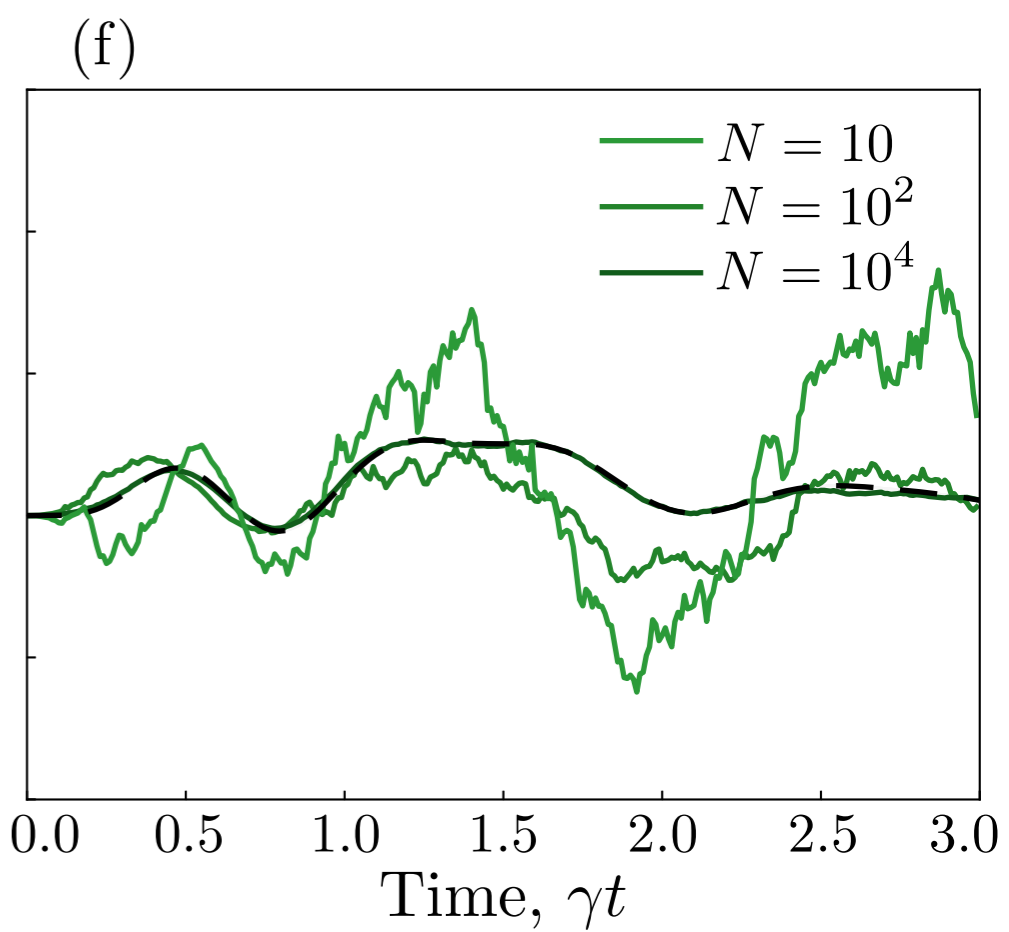

Supplement: Supplementary file 1 [file SM_Fig3.pdf]
