# Supplementary material for: Entanglement-Optimal Trajectories of Many-Body Quantum Markov Processes
Source: arXiv:2111.12048 source file (2022-05-16)

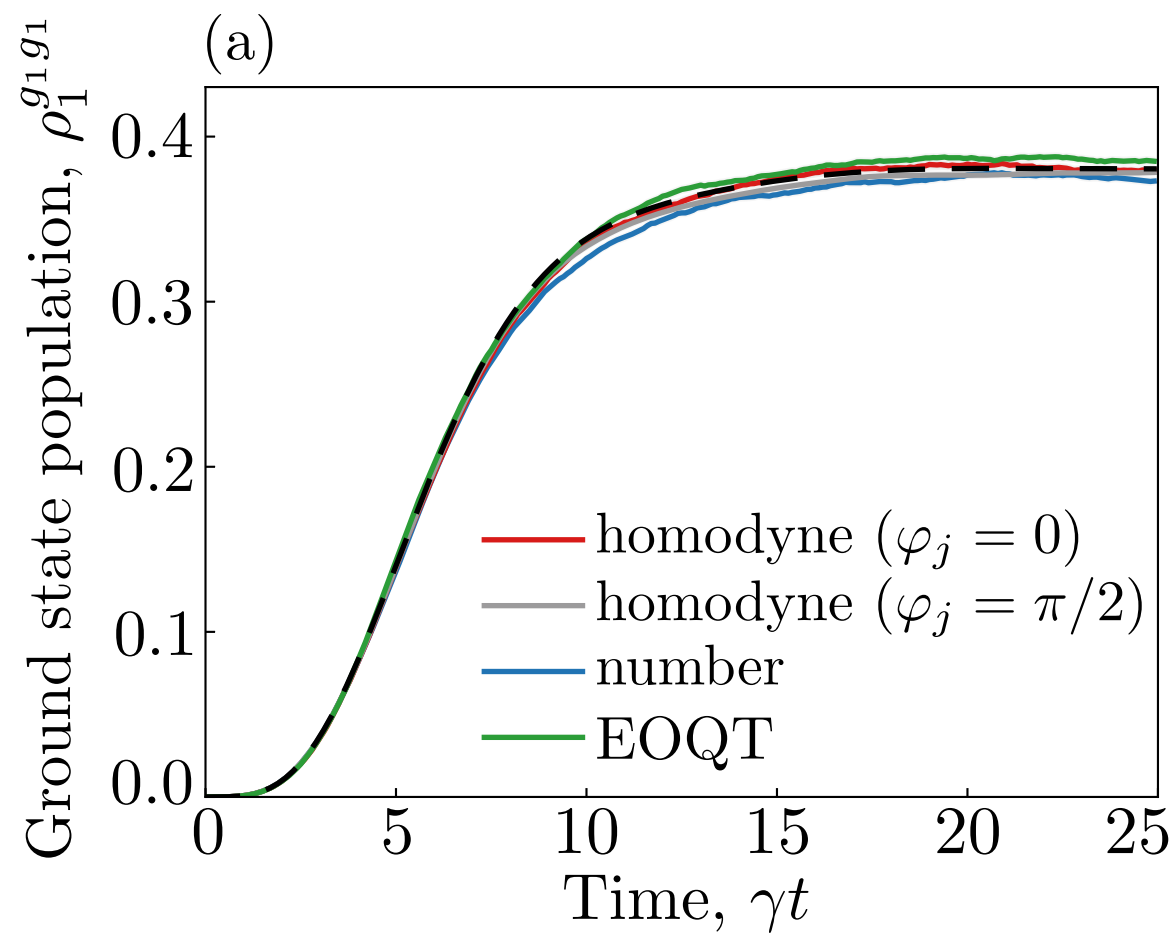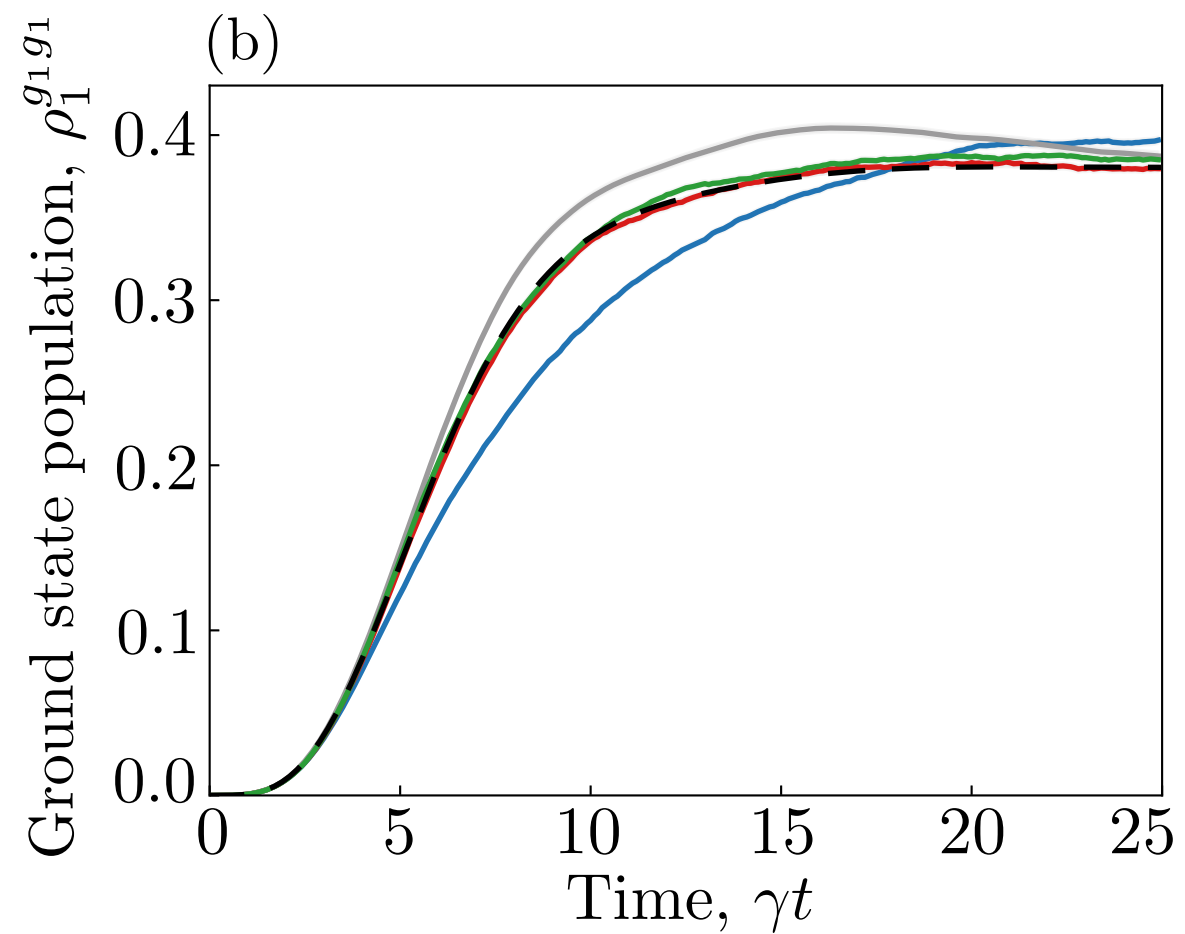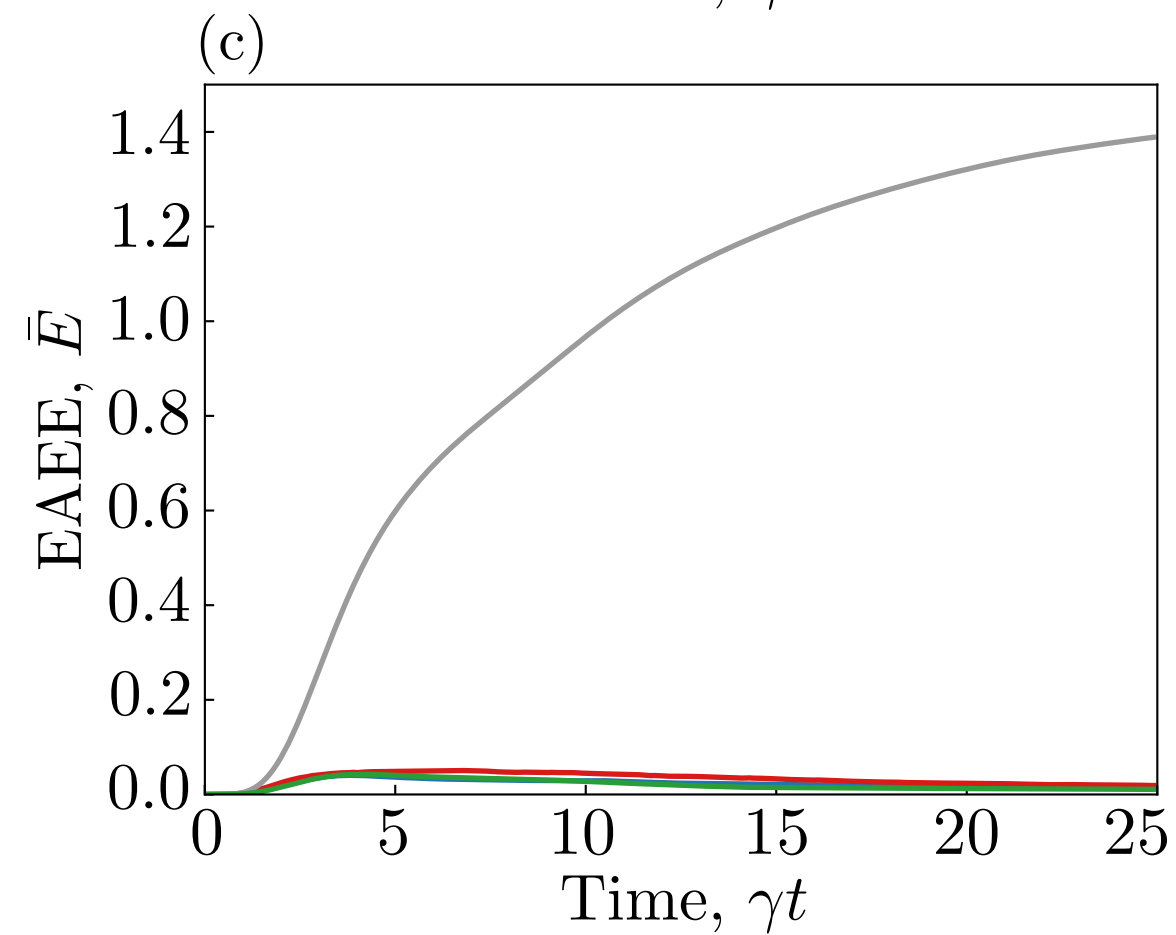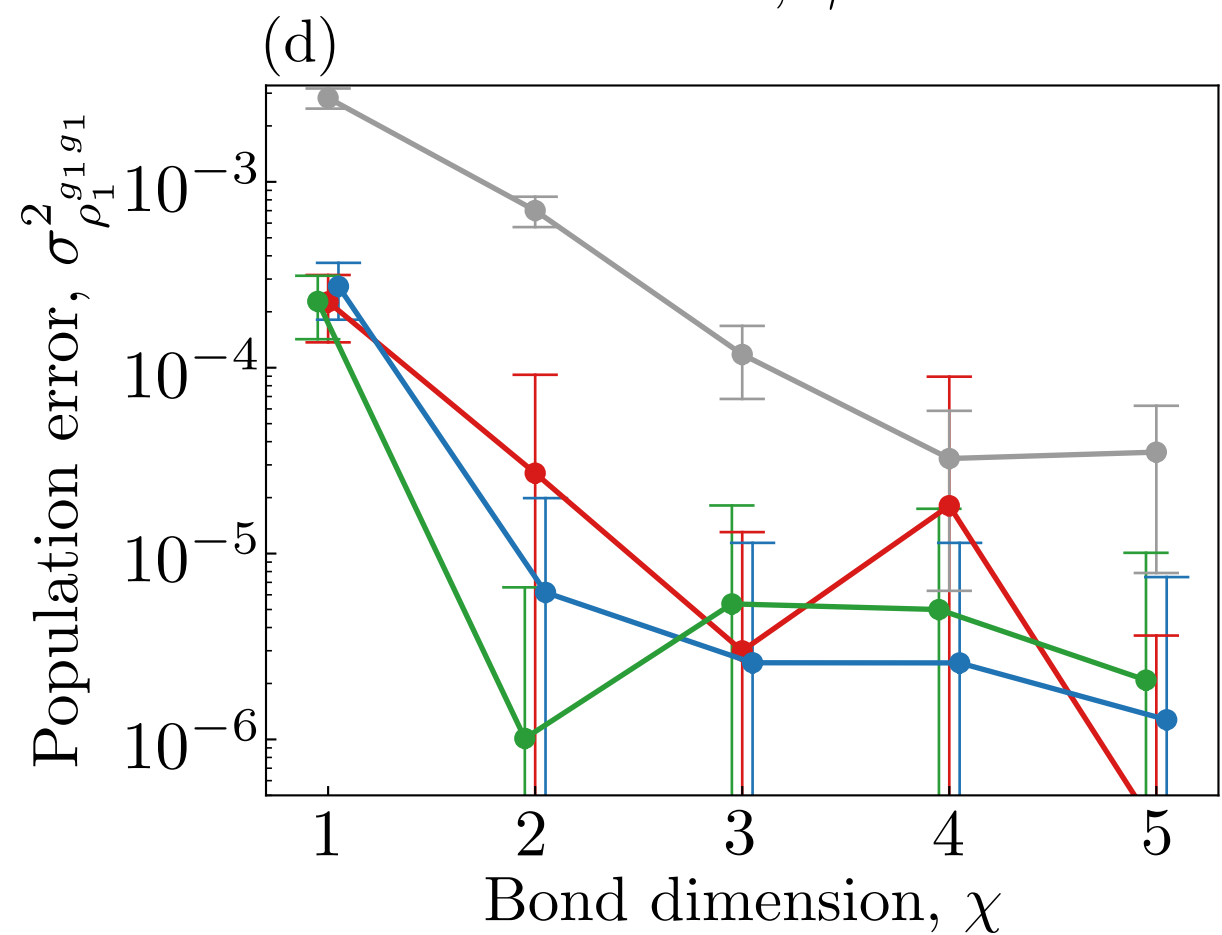

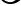

Supplement: Supplementary file 2 [file SM_Fig5.pdf]
